# Supplementary material for: Coulomb enhancement of superconducting pair-pair correlations in a $\frac{3}{4}$-filled model for $\kappa$-(BEDT-TTF)$_2$X
Source: arXiv:1602.08480 ancillary file (2016-02-26)
Supplement: Supplementary file 1 [file supplemental-02-23-2016.pdf]

# Supplemental Material for "Coulomb enhancement of superconducting pair-pair correlations in a $\frac{3}{4}$-filled model for $\kappa$-(BEDT-TTF)$_2$X"

W. Wasanthi De Silva,[1] Niladri Gomes,[2] S. Mazumdar,[2] and R. Torsten Clay[1]

[1]*Department of Physics and Astronomy and HPC$^2$ Center for Computational Sciences, Mississippi State, MS 39762*
[2]*Department of Physics, University of Arizona, Tucson, AZ 85721*

(Dated: February 23, 2016)

## S.1. LATTICES AND PAIRING SYMMETRIES

Fig. S1 shows the two lattices we considered. The **a** and **c** crystal axes shown are for $\kappa$-(BEDT-TTF)$_2$Cu[N(CN)$_2$]Cl; for $\kappa$-(BEDT-TTF)$_2$Cu$_2$(CN)$_3$ the corresponding axes are conventionally taken as **b** and **c**. We used the tight-binding hopping integrals calculated in Reference 60, which for $\kappa$-(BEDT-TTF)$_2$Cu[N(CN)$_2$]Cl are $t_{b1} = 207$ meV, $t_{b2} = 67$ meV, $t_p = -102$ meV, and $t_q = -43$ meV. For $\kappa$-(BEDT-TTF)$_2$Cu$_2$(CN)$_3$ $t_{b1} = 199$ meV, $t_{b2} = 91$ meV, $t_p = -85$ meV, and $t_q = -17$ meV.

The particular lattices were chosen to fulfill two requirements: (i) they are periodic, and (ii) in terms of the equivalent effective dimer model, an ordered Néel state is possible. The 32 site lattice we chose can be mapped to a 4×4 effective dimer model; the 64 site lattice to a 8×4 effective dimer model. In the following section, we explain the calculations of the enhancement of pair-pair correlations (Figs. 4 and 5 in the main paper). We show the full $U$ dependence for the average long-range pair-pair correlations ($\bar{P}$ as defined in the main paper) for each lattice, every carrier density, and each of the four $d$-wave pairing symmetries we considered.

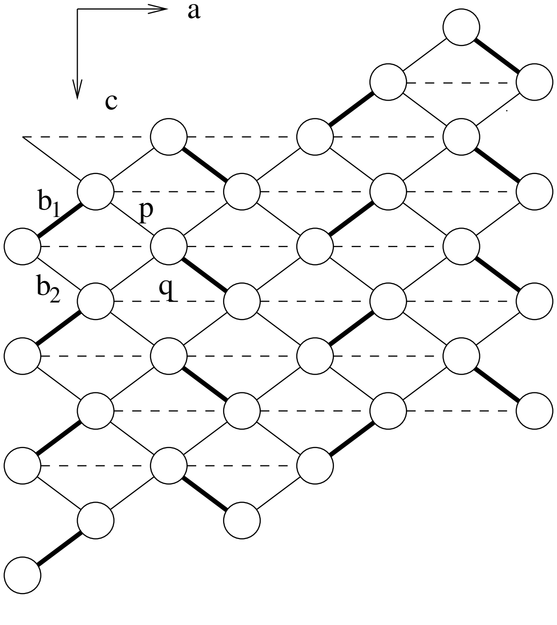


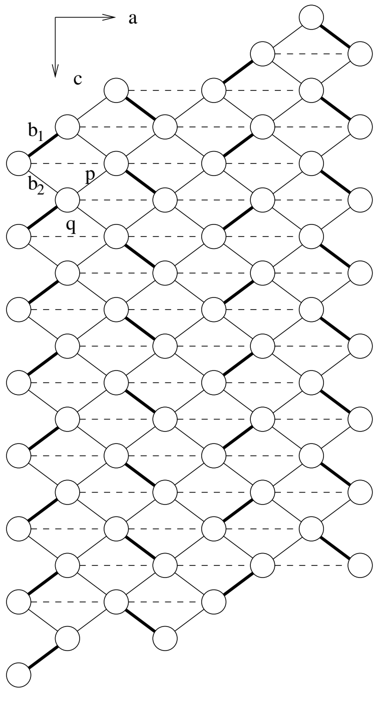


FIG. S1: (left) 32 site and (right) 64 site $\kappa$-(BEDT-TTF)$_2$X lattices.

## S.2. ENHANCEMENT OF PAIR-PAIR CORRELATIONS

In order to compare the enhancement of correlations with $U$ at different densities, we compute the normalized enhancement $\Theta_P = [\bar{P}(U)/\bar{P}(U=0)] - 1$. This normalization fails when the $U = 0$ correlations are identically zero, a finite-size effect. Very small $U = 0$ correlations also pose a problem. Therefore, in plotting $\Theta_P$ versus $\rho$ it is therefore necessary to exclude some specific $\rho$. The criteria we used for removing points in plots of $\Theta_P$ are follows:

1. A small value of $\bar{P}(U = 0)$ for all $U$, less than 0.0005 for 32 sites, and less than 0.0001 for 64 sites.
2. Results with $\bar{P} < 0$.
3. $\bar{P}$ changing discontinuously at large, finite $U$, indicating a quantum phase transition. This occurred at only one single point, for $\kappa$-Cl, $N = 32$, $N_e$=38, and is possibly related to a singlet-triplet transition or other finite-size effect. Note further than in several cases, particularly for some $\rho$ with $U = 0$ Fermi-level degeneracies, a discontinuous transition occurs for small $U$. See for example $N_e = 46$ in Fig. S9 or $N_e = 40$ in Fig. S12. In these cases, we used a value of $U$ *above the transition* rather than $U = 0$ for the normalization denominator in $\Theta_p$. In all cases the reference $U$ taken was $\leq 0.1$ eV.

The tables below list the data points that were excluded from Figs 4 and 5 in the main paper. They also show the reasons why these points were excluded.

### S.2.1. Fig. 4: $\kappa$-Cl

**$\rho$ removed, $\kappa$-Cl, $d_1$ (Fig. 4(a))**

| $N$ | $N_e$ | $\rho$ | Data Fig. | $\bar{P}$ magnitude | $\bar{P} < 0$ | discontinuity |
|---|---|---|---|---|---|---|
| 32 | 32 | 1.0000 | S2 | 0.0002 | | |
| 32 | 38 | 1.1875 | S2 | 0.0028 | ✓ | ✓ |
| 32 | 44 | 1.3750 | S2 | 0.0005 | ✓ | |
| 32 | 58 | 1.8125 | S3 | 0.0007 | ✓ | |
| 32 | 62 | 1.9375 | S3 | 0.0000 | | |
| 64 | 122 | 1.9063 | S19 | 0.00002 | | |
| 64 | 126 | 1.9688 | S19 | 0.0000 | | |

**$\rho$ removed, $\kappa$-Cl, $d_2$ (Fig. 4(b))**

| $N$ | $N_e$ | $\rho$ | Data Fig. | $\bar{P}$ magnitude | $\bar{P} < 0$ | discontinuity |
|---|---|---|---|---|---|---|
| 32 | 34 | 1.0625 | S4 | 0.002 | ✓ | |
| 32 | 36 | 1.1250 | S4 | 0.0002 | ✓ | |
| 32 | 38 | 1.1875 | S4 | 0.004 | ✓ | ✓ |
| 32 | 52 | 1.6250 | S5 | 0.002 | ✓ | |
| 32 | 54 | 1.6875 | S5 | 0.002 | ✓ | |
| 32 | 56 | 1.7500 | S5 | 0.002 | ✓ | |
| 32 | 58 | 1.8125 | S5 | 0.004 | ✓ | |
| 64 | 64 | 1.0000 | S20 | 0.00013 | ✓ | |
| 64 | 66 | 1.0313 | S20 | 0.0003 | ✓ | |
| 64 | 70 | 1.0938 | S20 | 0.0006 | ✓ | |
| 64 | 74 | 1.1563 | S20 | 0.00006 | ✓ | |

**$\rho$ removed, $\kappa$-Cl, $d_3$ (Fig. 4(c))**

| $N$ | $N_e$ | $\rho$ | Data Fig. | $\bar{P}$ magnitude | $\bar{P} < 0$ | discontinuity |
|---|---|---|---|---|---|---|
| 32 | 32 | 1.0000 | S6 | 0.0003 | ✓ | |
| 32 | 34 | 1.0625 | S6 | 0.0003 | | |
| 32 | 38 | 1.1875 | S6 | 0.001 | | ✓ |
| 32 | 58 | 1.8125 | S7 | 0.00007 | ✓ | |
| 64 | 64 | 1.0000 | S22 | 0.0003 | ✓ | |
| 64 | 66 | 1.0313 | S22 | 0.0002 | ✓ | |
| 64 | 70 | 1.0938 | S22 | 0.0003 | ✓ | |
| 64 | 74 | 1.1563 | S22 | 0.0005 | | |
| 64 | 122 | 1.9063 | S22 | 0.00006 | | |

Note that $N = 64$, $N_e = 102$ ($\rho = 1.5938$) was not removed in Fig. 4(c); here $\Theta_P$ is very close to zero ($\approx 0.0008$).

**$\rho$ removed, $\kappa$-Cl, $d_4$ (Fig. 4(d))**

| $N$ | $N_e$ | $\rho$ | Data Fig. | $\bar{P}$ magnitude | $\bar{P} < 0$ | discontinuity |
|---|---|---|---|---|---|---|
| 32 | 32 | 1.0000 | S8 | 0.0003 | ✓ | |
| 32 | 38 | 1.1875 | S8 | 0.001 | ✓ | ✓ |
| 32 | 58 | 1.8125 | S8 | 0.0004 | ✓ | |
| 64 | 64 | 1.0000 | S24 | 0.0001 | ✓ | |
| 64 | 102 | 1.5938 | S24 | 0.00007 | | |

### S.2.2. Fig. 5: $\kappa$-CN

**$\rho$ removed, $\kappa$-CN, $d_1$ (Fig. 5(a))**

| $N$ | $N_e$ | $\rho$ | Data Fig. | $\bar{P}$ magnitude | $\bar{P} < 0$ | discontinuity |
|---|---|---|---|---|---|---|
| 32 | 32 | 1.0000 | S10 | 0.00007 | ✓ | |
| 32 | 56 | 1.7500 | S11 | 0.0007 | ✓ | |
| 32 | 58 | 1.8125 | S11 | 0.0007 | ✓ | |
| 32 | 62 | 1.9375 | S11 | 0.0000 | | |
| 64 | 64 | 1.0000 | S26 | 0.00002 | ✓ | |
| 64 | 122 | 1.9063 | S27 | 0.00002 | | |
| 64 | 126 | 1.9688 | S27 | 0.00000 | | |

**$\rho$ removed, $\kappa$-CN, $d_2$ (Fig. 5(b))**

| $N$ | $N_e$ | $\rho$ | Data Fig. | $\bar{P}$ magnitude | $\bar{P} < 0$ | discontinuity |
|---|---|---|---|---|---|---|
| 32 | 34 | 1.0625 | S12 | 0.0004 | ✓ | |
| 32 | 36 | 1.1250 | S12 | 0.0015 | ✓ | |
| 32 | 38 | 1.1875 | S12 | 0.0025 | ✓ | |
| 32 | 40 | 1.2500 | S12 | 0.001 | ✓ | |
| 32 | 42 | 1.3125 | S12 | 0.001 | ✓ | |
| 32 | 44 | 1.3750 | S12 | 0.001 | ✓ | |
| 32 | 46 | 1.4375 | S13 | 0.001 | ✓ | |
| 32 | 48 | 1.5000 | S13 | 0.001 | ✓ | |
| 32 | 52 | 1.6250 | S13 | 0.0005 | ✓ | |
| 32 | 54 | 1.6875 | S13 | 0.0015 | ✓ | |
| 32 | 56 | 1.7500 | S13 | 0.005 | ✓ | |
| 32 | 58 | 1.8125 | S13 | 0.005 | ✓ | |
| 64 | 64 | 1.0000 | S29 | 0.0001 | ✓ | |
| 64 | 78 | 1.2188 | S29 | 0.00003 | ✓ | |
| 64 | 82 | 1.2813 | S29 | 0.0007 | ✓ | |
| 64 | 86 | 1.3438 | S29 | 0.00005 | ✓ | |

**$\rho$ removed, $\kappa$-CN, $d_3$ (Fig. 5(c))**

| $N$ | $N_e$ | $\rho$ | Data Fig. | $\bar{P}$ magnitude | $\bar{P} < 0$ | discontinuity |
|---|---|---|---|---|---|---|
| 32 | 56 | 1.7500 | S14 | 0.0003 | | |
| 32 | 58 | 1.8125 | S15 | 0.0001 | ✓ | |
| 64 | 64 | 1.0000 | S30 | 0.0004 | ✓ | |
| 64 | 68 | 1.0625 | S30 | 0.0004 | ✓ | |
| 64 | 70 | 1.09375 | S30 | 0.0003 | ✓ | |

**$\rho$ removed, $\kappa$-CN, $d_4$ (Fig. 5(d))**

| $N$ | $N_e$ | $\rho$ | Data Fig. | $\bar{P}$ magnitude | $\bar{P} < 0$ | discontinuity |
|---|---|---|---|---|---|---|
| 32 | 32 | 1.0000 | S16 | 0.00003 | ✓ | |
| 32 | 56 | 1.7500 | S16 | 0.0004 | ✓ | |
| 32 | 58 | 1.8125 | S17 | 0.0005 | ✓ | |
| 64 | 64 | 1.0000 | S32 | 0.0001 | ✓ | |

In the following we show plots of $\bar{P}(U)$ against $U$, for every carrier density, pairing symmetry, and lattice. In each case the thick horizontal line show the lower cutoff for $\bar{P}(U)$, data points below which have been excluded in Figs. 4 and 5 of main paper.

## S.3. 32 SITE LATTICE

### S.3.1. X=Cl, pairing symmetry $d_1$

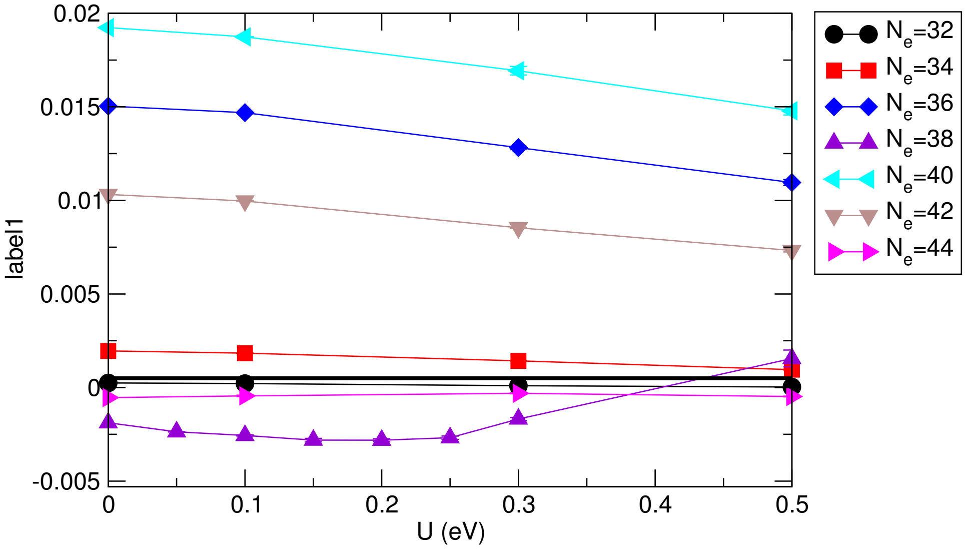


FIG. S2: PIRG average long-range pair-pair correlations for the 32 site lattice, X=Cl, symmetry $d_1$. Suppression of pair-pair correlations occurs for all $N_e$

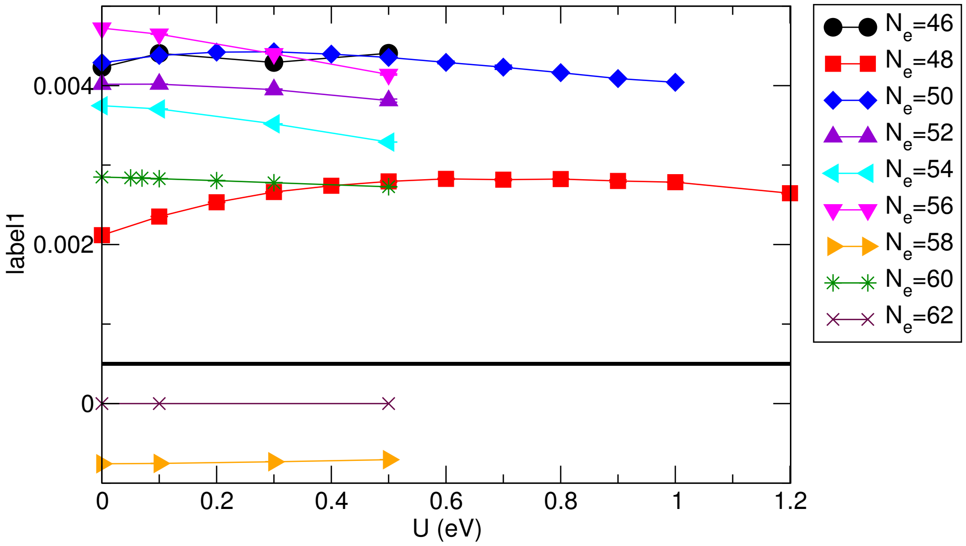


FIG. S3: PIRG average long-range pair-pair correlations for the 32 site lattice, X=Cl, symmetry $d_1$. Suppression of pair-pair correlations occurs for all $N_e$, except $N_e$ = 48 and 50. The strong enhancement at $N_e$=48 is shown in Fig. 4(a) of the main paper.

### S.3.2. X=Cl, pairing symmetry $d_2$

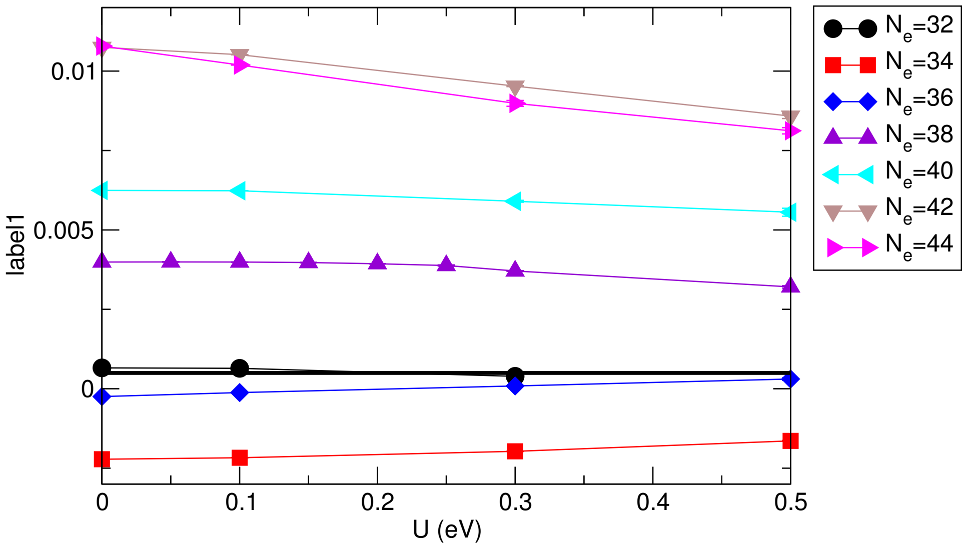


FIG. S4: PIRG average long-range pair-pair correlations for the 32 site lattice, X=Cl, symmetry $d_2$. Suppression of pair-pair correlations occurs for all $N_e$.

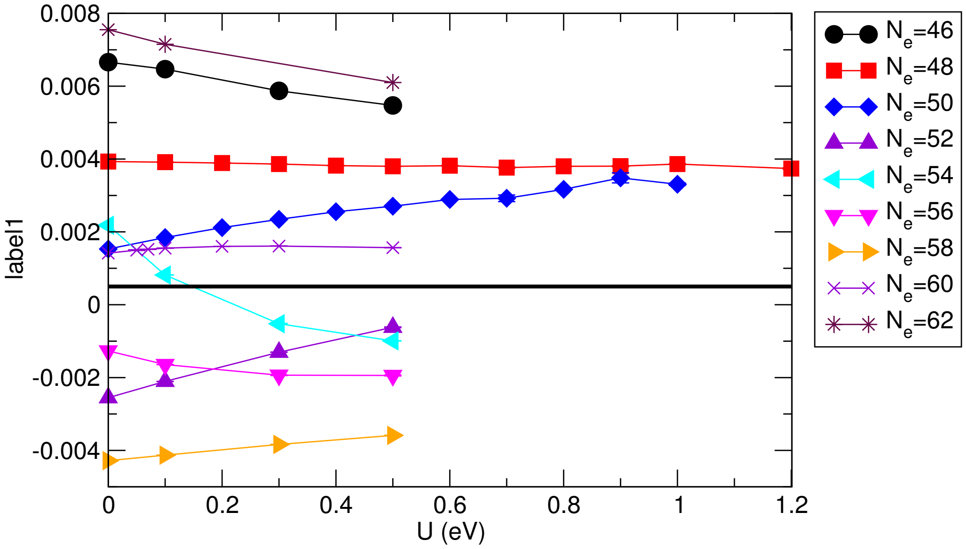


FIG. S5: PIRG average long-range pair-pair correlations for the 32 site lattice, X=Cl, symmetry $d_2$. Suppression of pair-pair correlations occurs for all $N_e$ except $N_e = 50$. The strong enhancement at $N_e = 50$ is shown in Fig. 4(b) of the main paper.

### S.3.3. X=Cl, pairing symmetry $d_3$

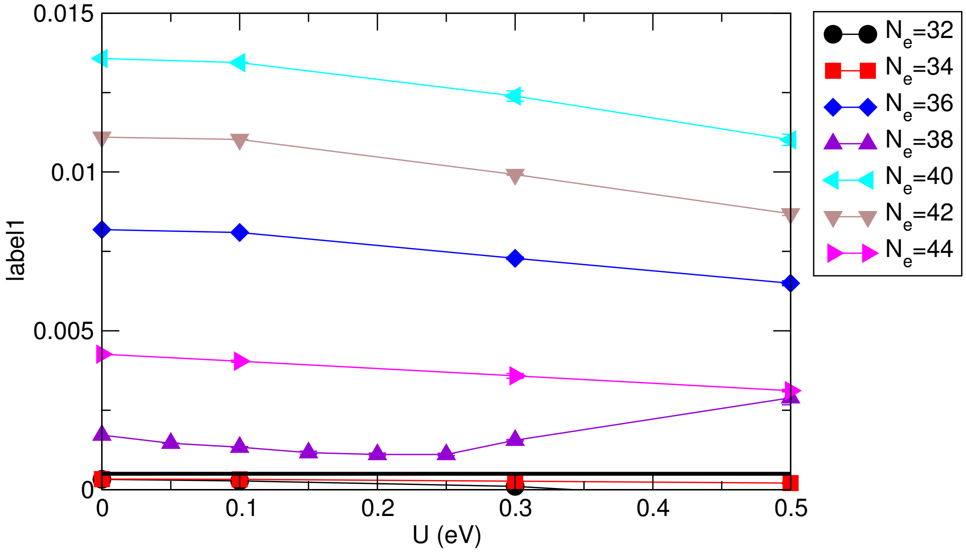


FIG. S6: PIRG average long-range pair-pair correlations for the 32 site lattice, X=Cl, symmetry $d_3$. Suppression of pair-pair correlations occurs for all $N_e$.

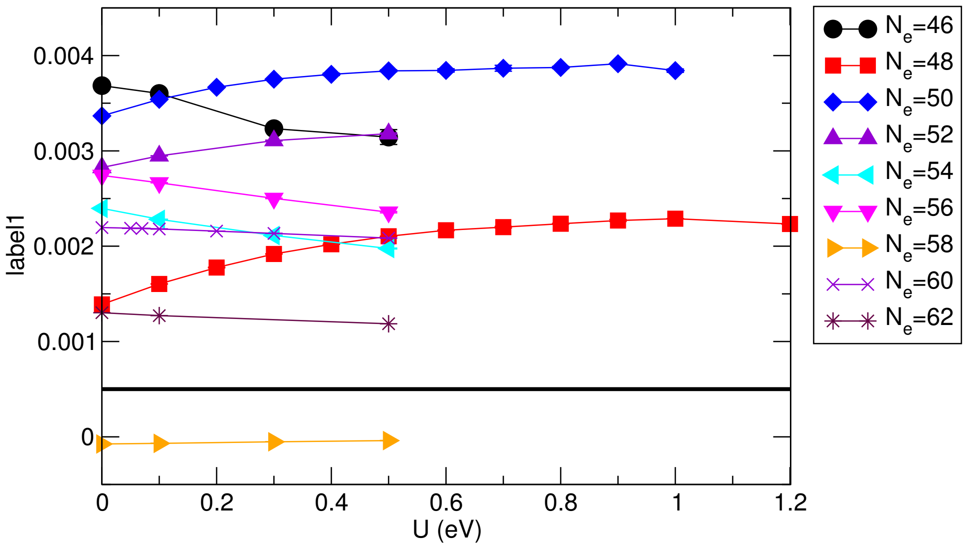


FIG. S7: PIRG average long-range pair-pair correlations for the 32 site lattice, X=Cl, symmetry $d_3$. Suppression of pair-pair correlations occurs for all $N_e$ except $N_e = 48, 50, 52$. The strong enhancement at $N_e = 48$ is shown in Fig. 4(c) of the main paper.

### S.3.4. X=Cl, pairing symmetry $d_4$

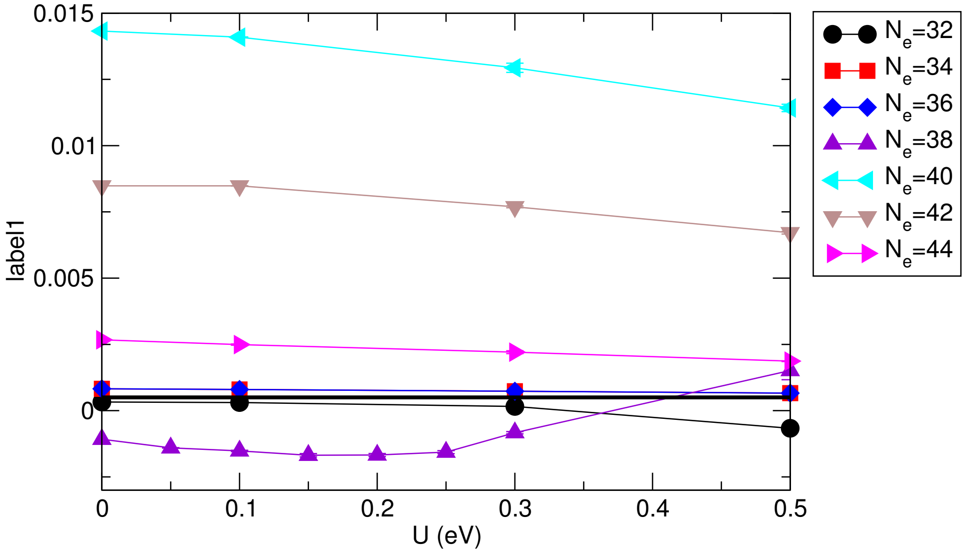


FIG. S8: PIRG average long-range pair-pair correlations for the 32 site lattice, X=Cl, symmetry $d_4$. Suppression of pair-pair correlations occurs for all $N_e$.

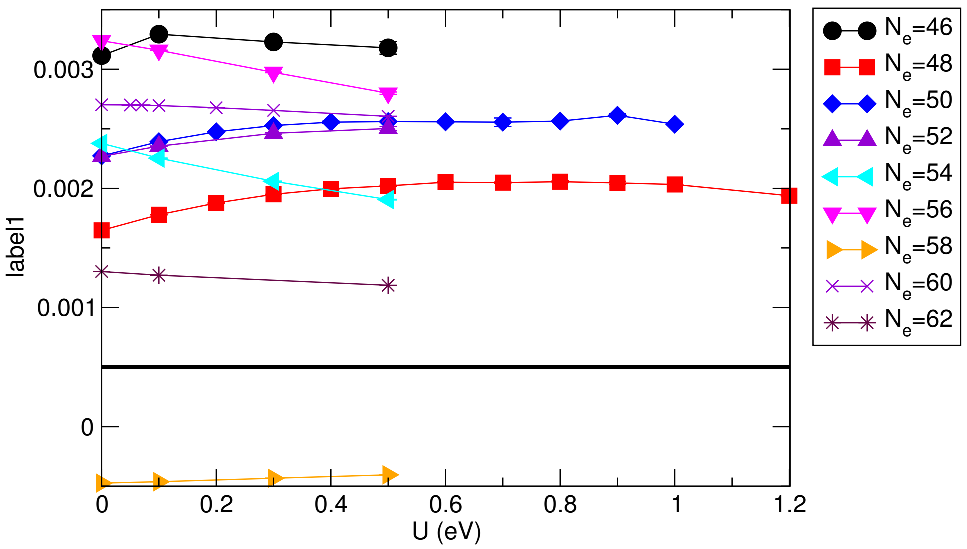


FIG. S9: PIRG average long-range pair-pair correlations for the 32 site lattice, X=Cl, symmetry $d_4$. Suppression of pair-pair correlations occurs for all $N_e$ except $N_e = 48, 50, 52$. These enhancements are indicated in Fig. 4(d) of main paper.

### S.3.5. X=CN, pairing symmetry $d_1$

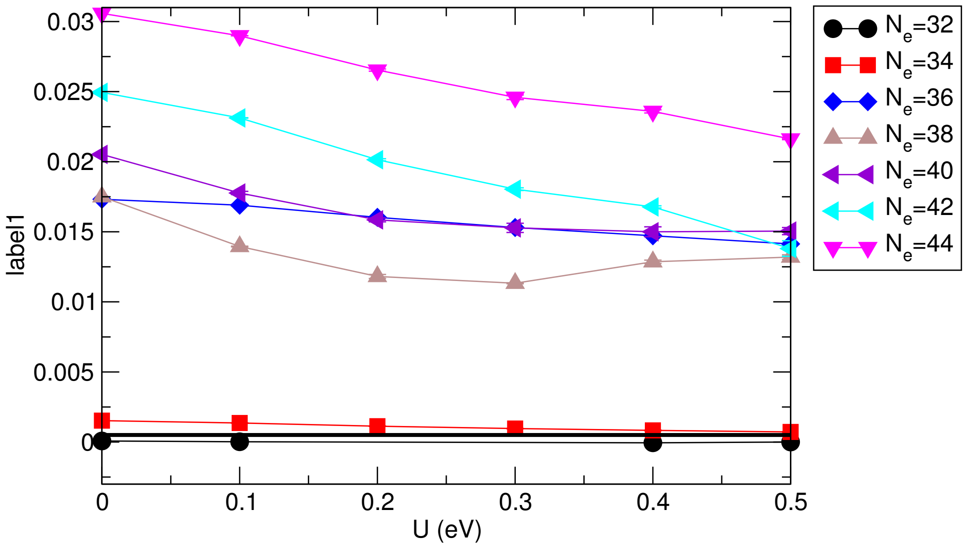


FIG. S10: PIRG average long-range pair-pair correlations for the 32 site lattice, X=CN, symmetry $d_1$. Suppression of pair-pair correlations occurs for all $N_e$.

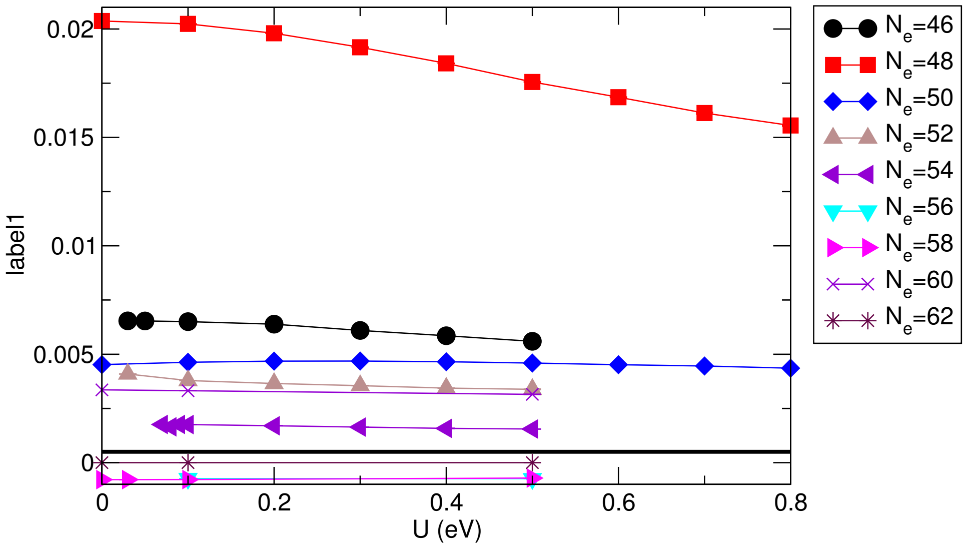


FIG. S11: PIRG average long-range pair-pair correlations for the 32 site lattice, X=CN, symmetry $d_1$. Suppression of pair-pair correlations occurs for all $N_e$.

### S.3.6. X=CN, pairing symmetry $d_2$

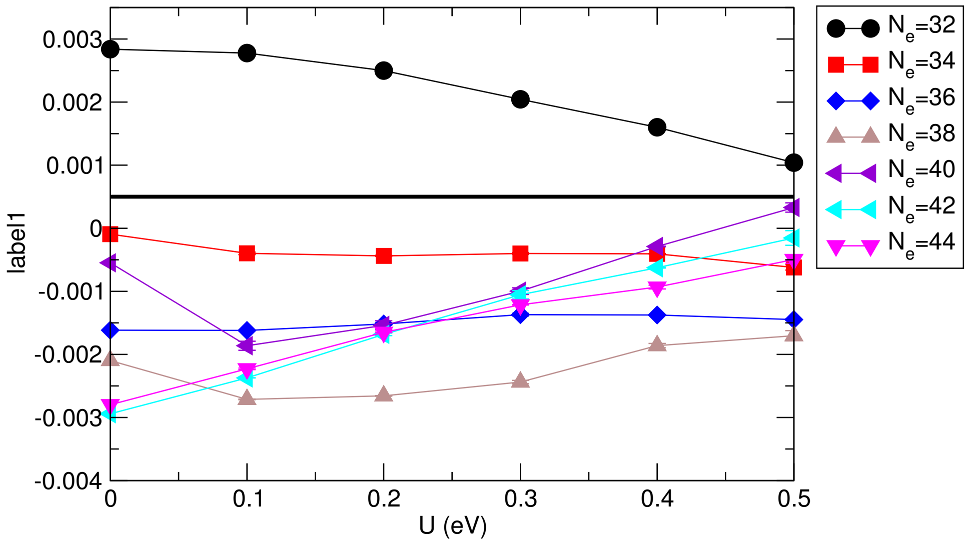


FIG. S12: PIRG average long-range pair-pair correlations for the 32 site lattice, X=CN, symmetry $d_2$. Suppression of pair-pair correlations occurs for $N_e = 32$, while $P(\bar{U})$ is negative for all other $N_e$.

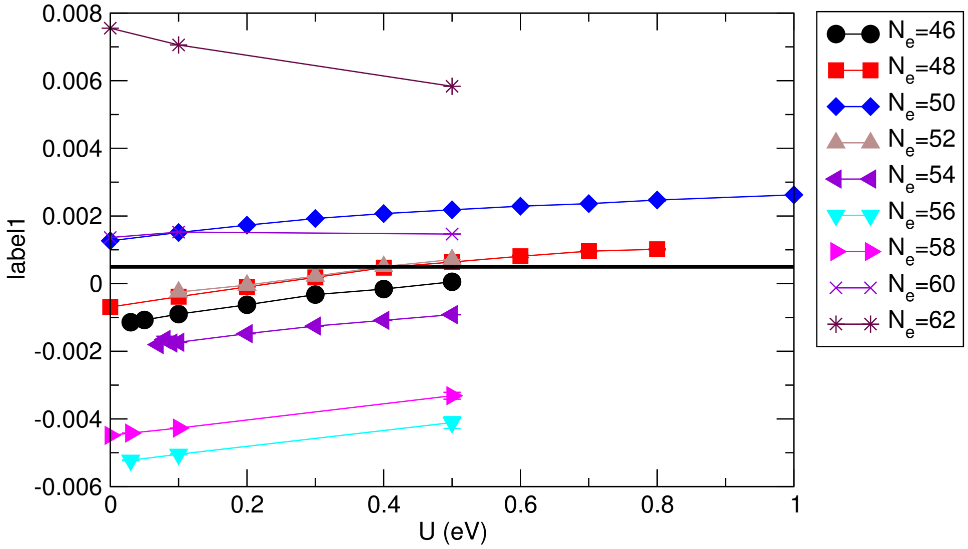


FIG. S13: PIRG average long-range pair-pair correlations for the 32 site lattice, X=CN, symmetry $d_2$. The strong enhancement for $N_e = 50$ is shown in Fig. 5(b) of the main paper. Note that the other densities close to $\rho = 1.5$, $N_e$=46, 48, and 52 are also enhanced, although we have not plotted the enhanced $\Theta_P$ in Fig. 5(b) due to the sign change with increasing $U$ in $\bar{P}$.

### S.3.7. X=CN, pairing symmetry $d_3$

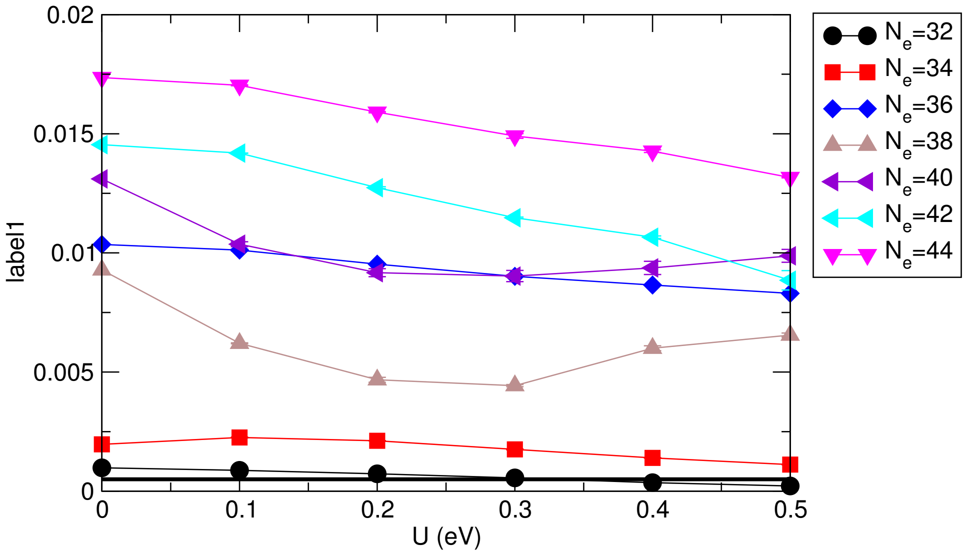


FIG. S14: PIRG average long-range pair-pair correlations for the 32 site lattice, X=CN, symmetry $d_3$. Suppression of pair-pair correlations occurs for $N_e$.

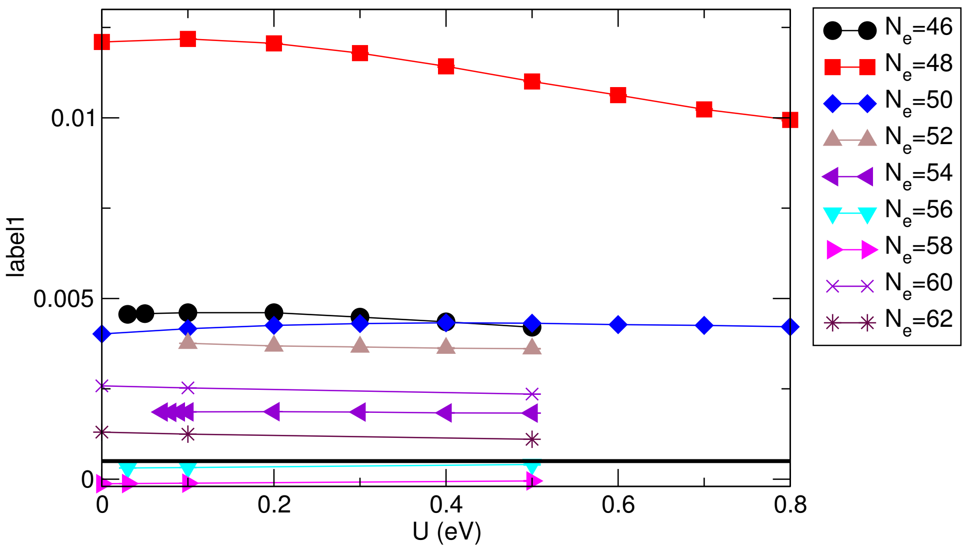


FIG. S15: PIRG average long-range pair-pair correlations for the 32 site lattice, X=CN, symmetry $d_3$. Suppression of pair-pair correlations occurs for $N_e$, except at $N_e = 50$, where weak enhancement occurs. This enhancement has been indicated in Fig. 5(c) of main paper.

### S.3.8. X=CN, pairing symmetry $d_4$

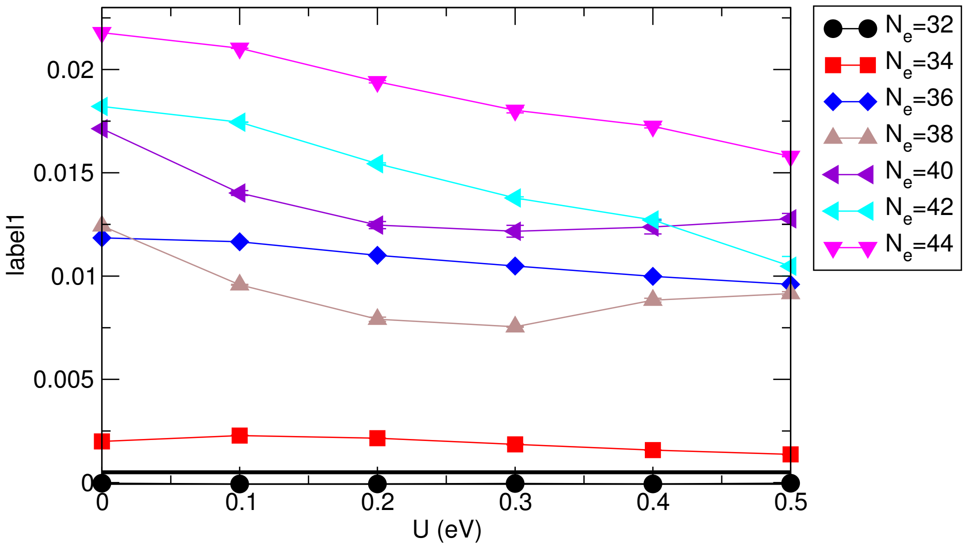


FIG. S16: PIRG average long-range pair-pair correlations for the 32 site lattice, X=CN, symmetry $d_4$. Suppression of pair-pair correlations occurs for $N_e$.

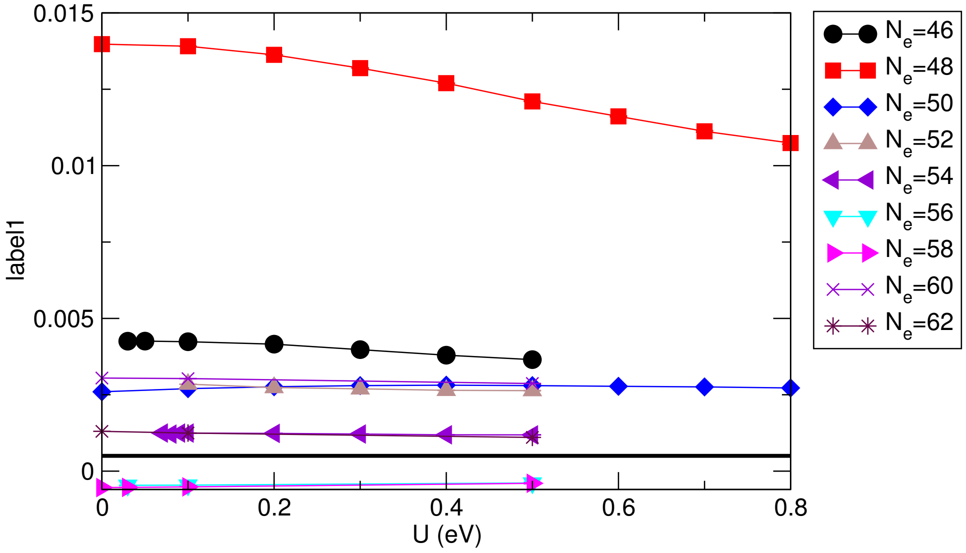


FIG. S17: PIRG average long-range pair-pair correlations for the 32 site lattice, X=CN, symmetry $d_4$. Suppression of pair-pair correlations occurs for $N_e$, except at $N_e = 50$, where weak enhancement occurs. This enhancement has been indicated in Fig. 5(d) of main paper.

## S.4. 64 SITE LATTICE

### S.4.1. X=Cl, pairing symmetry $d_1$

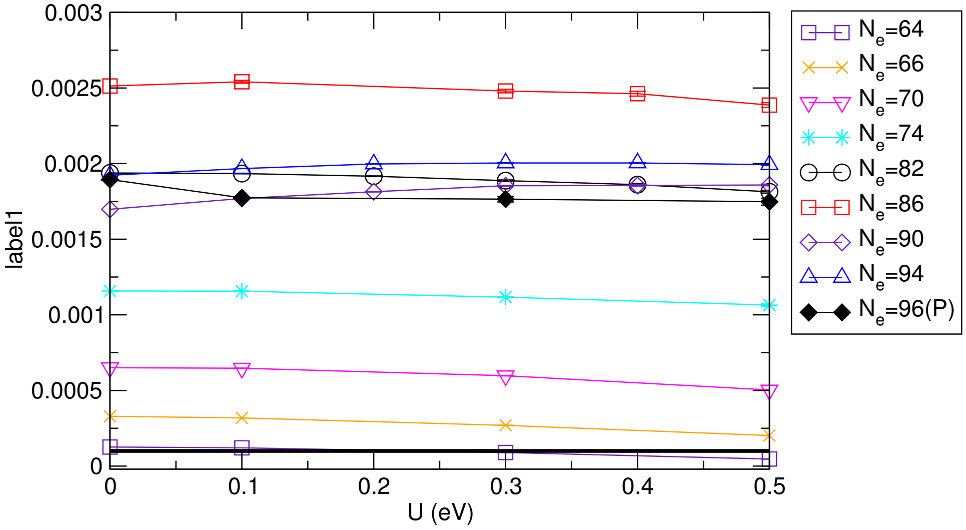


FIG. S18: CPMC average long-range pair-pair correlations for the 64 site lattice, X=Cl, symmetry $d_1$. Absence of enhancement in pair-pair correlations is seen for all $N_e$.

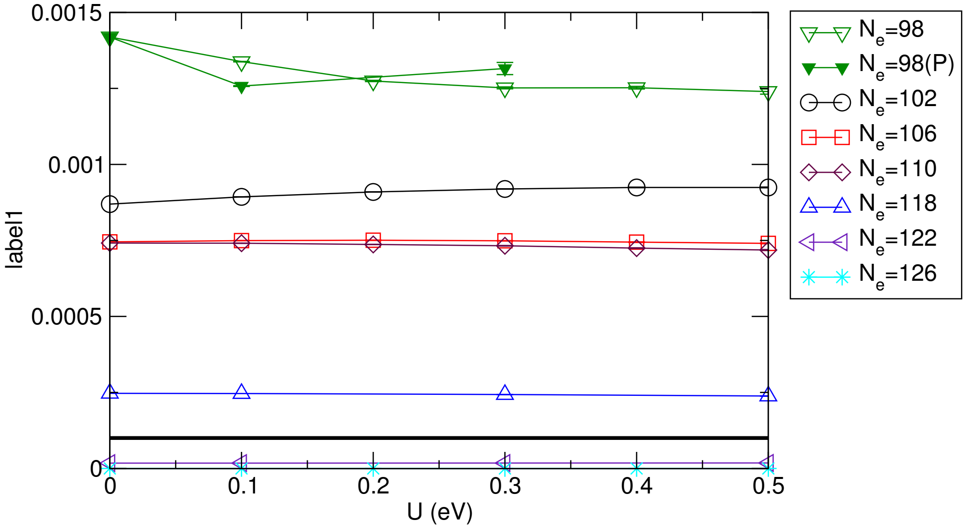


FIG. S19: CPMC average long-range pair-pair correlations for the 64 site lattice, X=Cl, symmetry $d_1$. Absence of enhancement in pair-pair correlations is seen for all $N_e$.

### S.4.2. X=Cl, pairing symmetry $d_2$

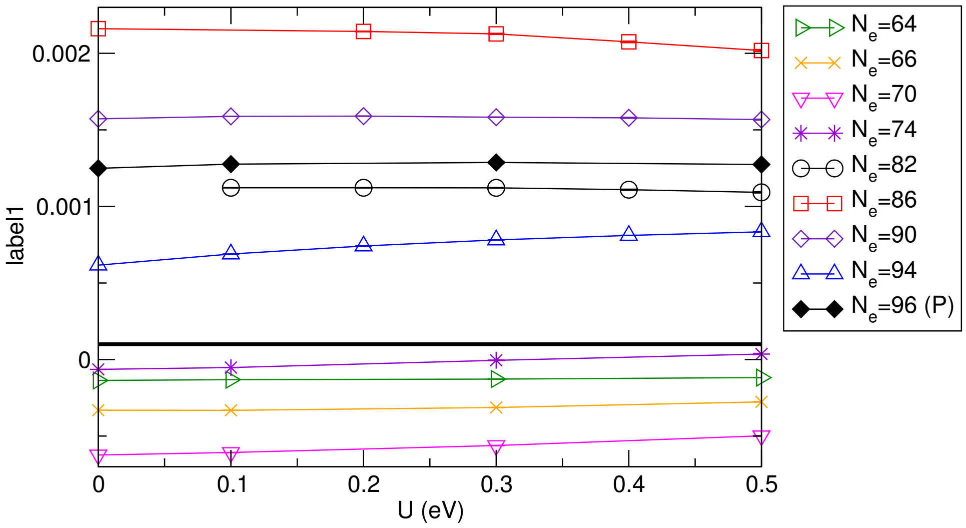


FIG. S20: CPMC average long-range pair-pair correlations for the 64 site lattice, X=Cl, symmetry $d_2$. Enhancement of pair-pair correlations is seen only for $N_e$=94 which is plotted in Fig. 6(c).

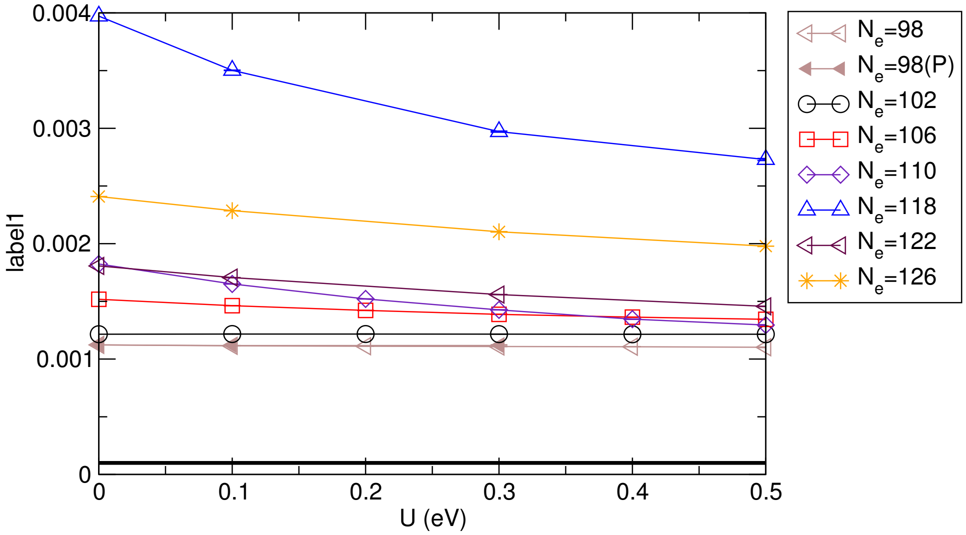


FIG. S21: CPMC average long-range pair-pair correlations for the 64 site lattice, X=Cl, symmetry $d_2$. Suppression of pair-pair correlations is seen only for $N_e$.

### S.4.3. X=Cl, pairing symmetry $d_3$

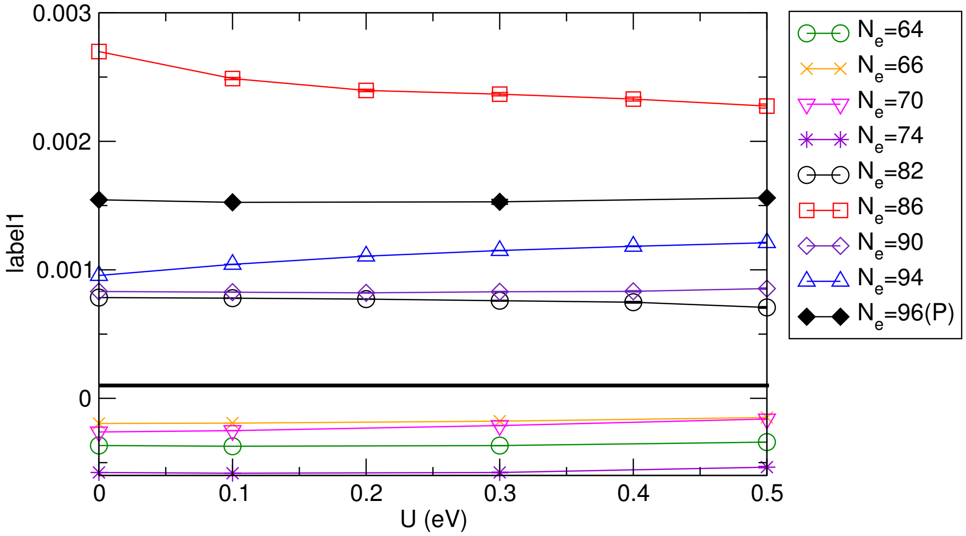


FIG. S22: CPMC average long-range pair-pair correlations for the 64 site lattice, X=Cl, symmetry $d_3$. Enhancement of pair-pair correlations is seen only for $N_e = 94$ which is plotted in Fig. 6(c).

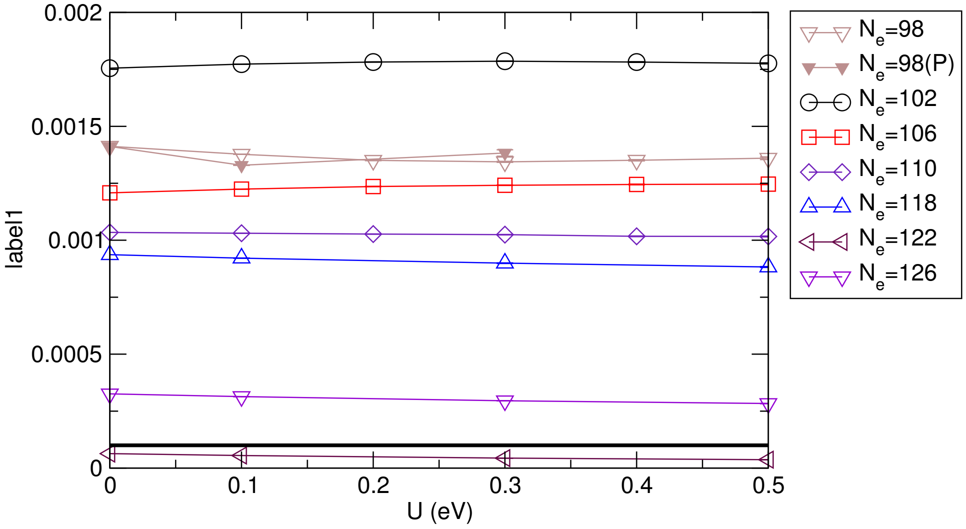


FIG. S23: CPMC average long-range pair-pair correlations for the 64 site lattice, X=Cl, symmetry $d_3$. Suppression of pair-pair correlations is seen for all $N_e$.

### S.4.4. X=Cl, pairing symmetry $d_4$

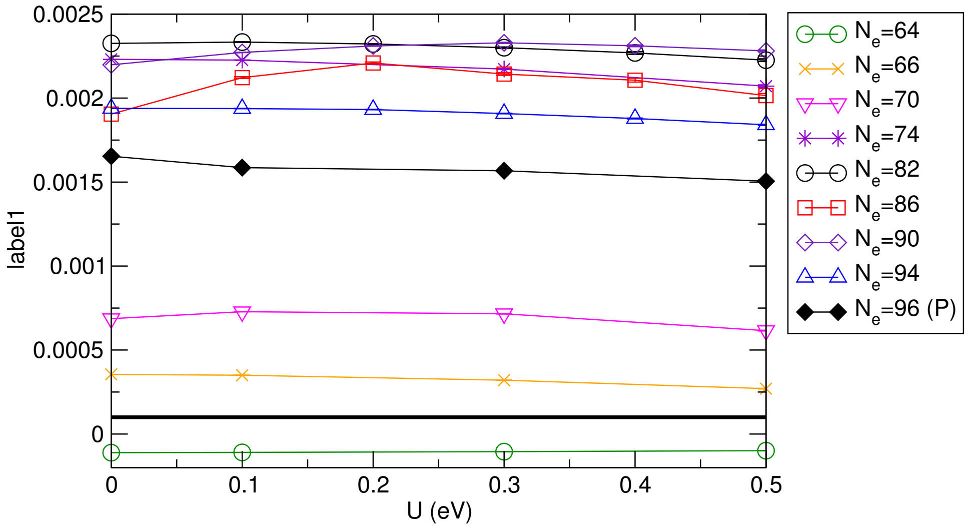


FIG. S24: CPMC average long-range pair-pair correlations for the 64 site lattice, X=Cl, symmetry $d_4$. Absence of enhancement is seen for all $N_e$.

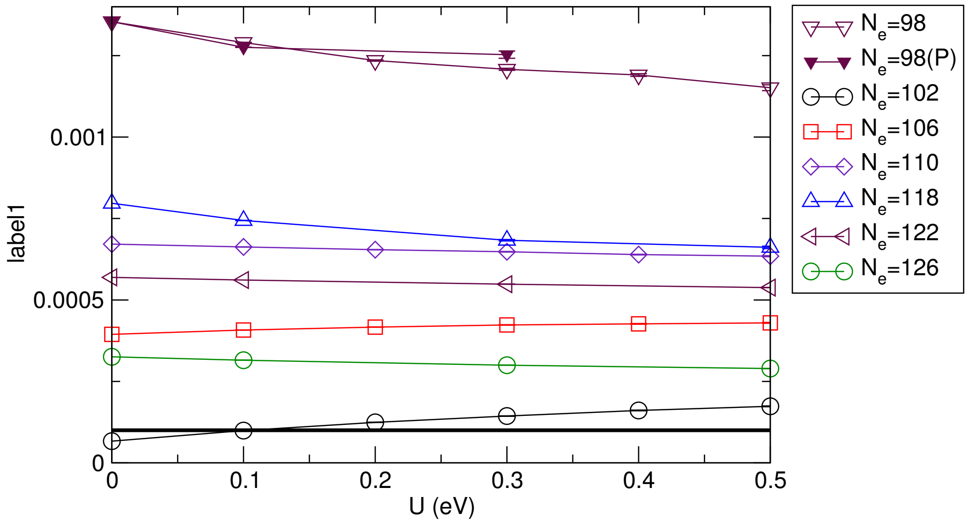


FIG. S25: CPMC average long-range pair-pair correlations for the 64 site lattice, X=Cl, symmetry $d_4$. Suppression pair-pair correlations is seen for all $N_e$ except $N_e = 102$, where a change of sign occurs.

### S.4.5. X=CN, pairing symmetry $d_1$

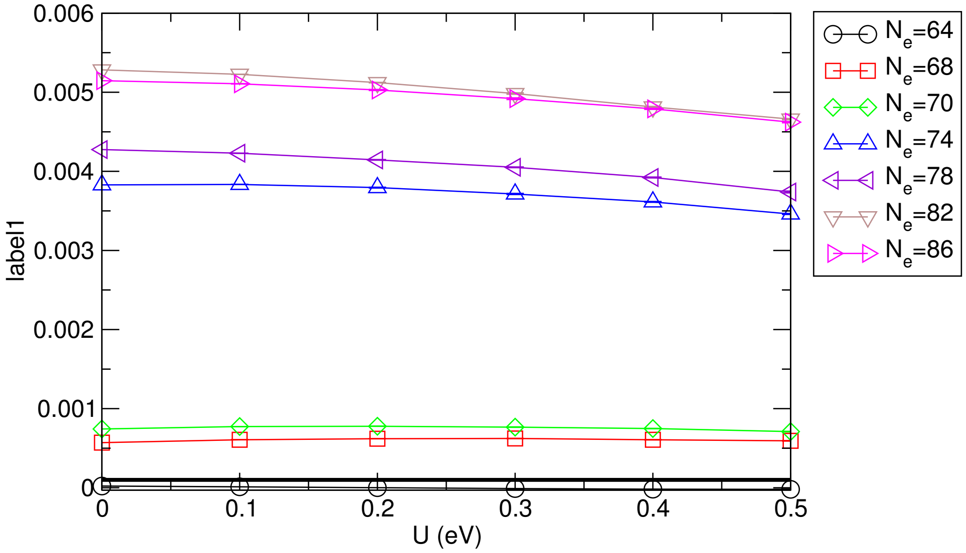


FIG. S26: CPMC average long-range pair-pair correlations for the 64 site lattice, X=CN, symmetry $d_1$. Suppression pair-pair correlations is seen for all $N_e$.

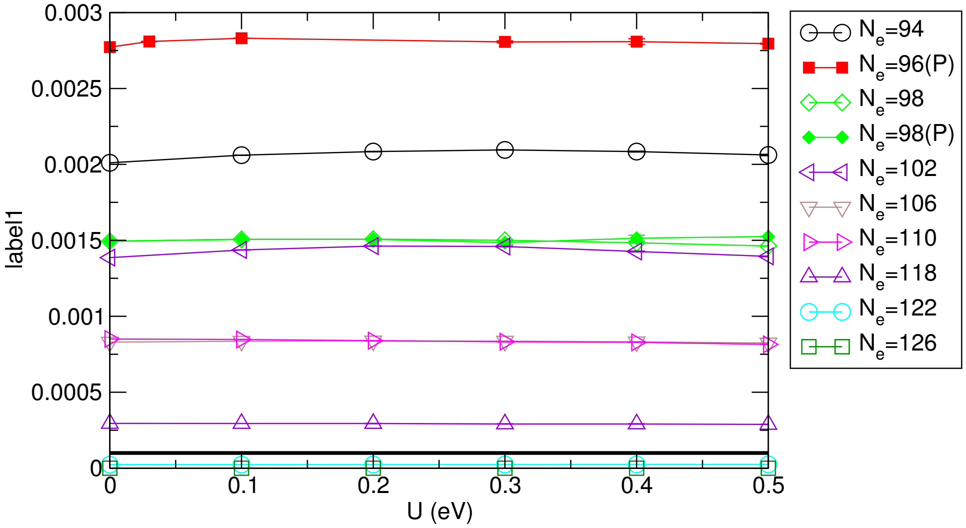


FIG. S27: CPMC average long-range pair-pair correlations for the 64 site lattice, X=CN, symmetry $d_1$. Absence of enhancement of pair-pair correlations is seen for all $N_e$.

### S.4.6. X=CN, pairing symmetry $d_2$

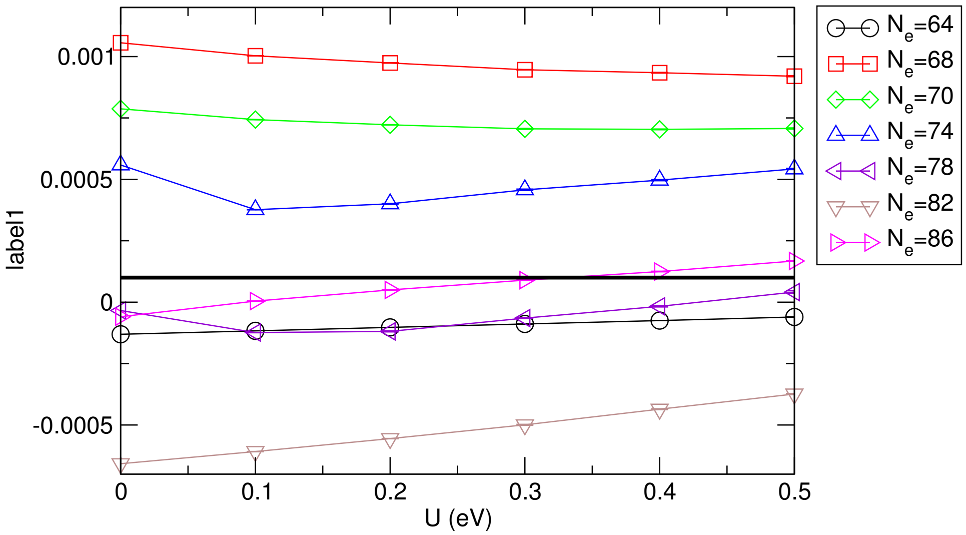


FIG. S28: CPMC average long-range pair-pair correlations for the 64 site lattice, X=CN, symmetry $d_2$. Absence of enhancement is seen for all $N_e$.

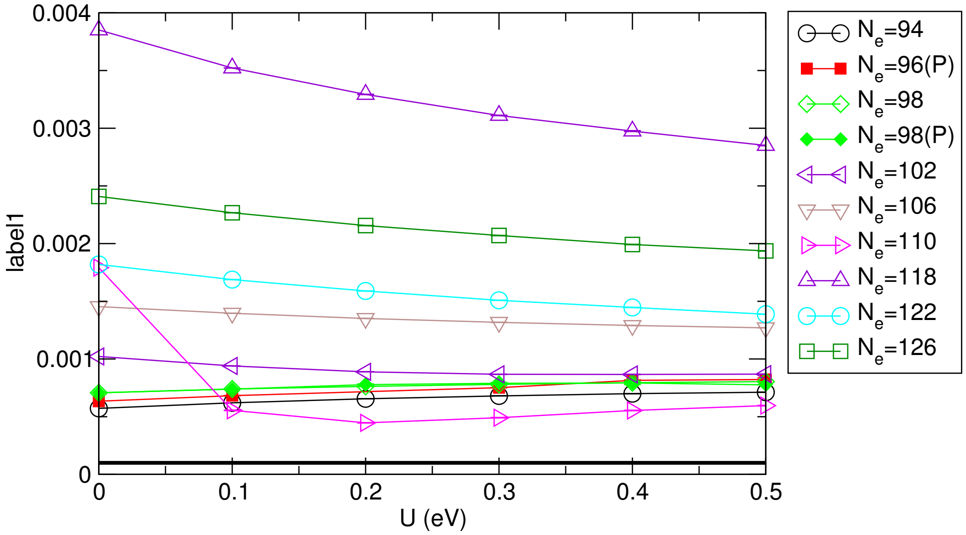


FIG. S29: CPMC average long-range pair-pair correlations for the 64 site lattice, X=CN, symmetry $d_2$. Enhancement is seen only for $N_e = 96$ and 98 which are plotted in Fig. 6(d).

### S.4.7. X=CN, pairing symmetry $d_3$

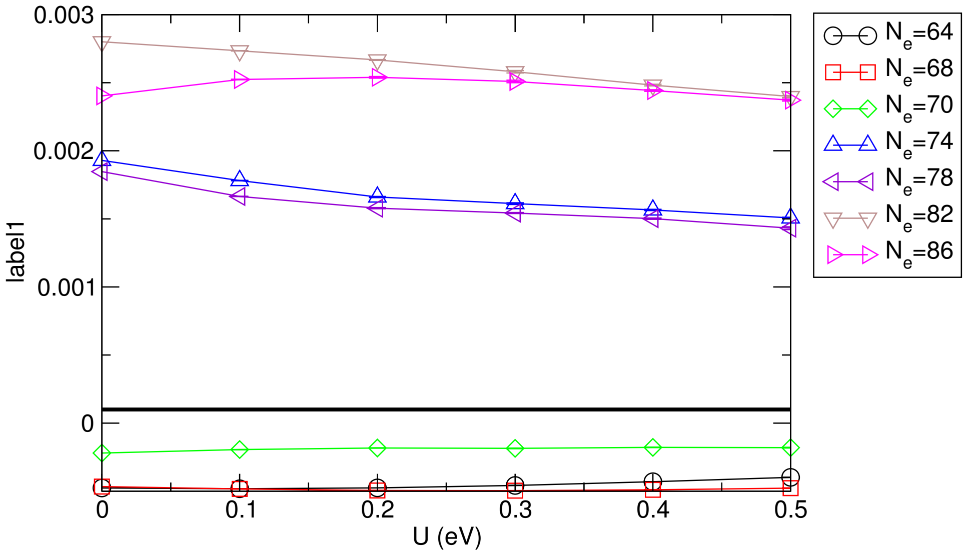


FIG. S30: CPMC average long-range pair-pair correlations for the 64 site lattice, X=CN, symmetry $d_3$. Absence of enhancement is seen for all $N_e$.

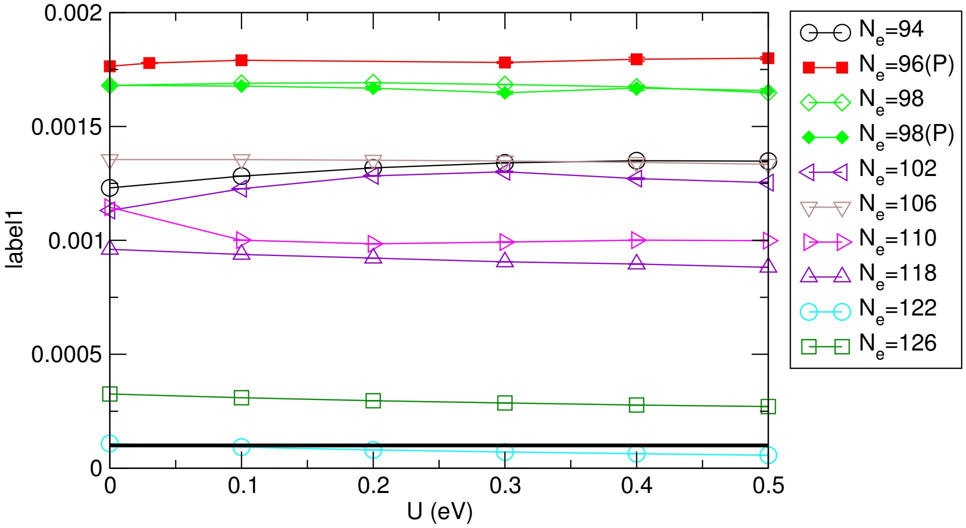


FIG. S31: CPMC average long-range pair-pair correlations for the 64 site lattice, X=CN, symmetry $d_3$. Absence of enhancement is seen for all $N_e$.

### S.4.8. X=CN, pairing symmetry $d_4$

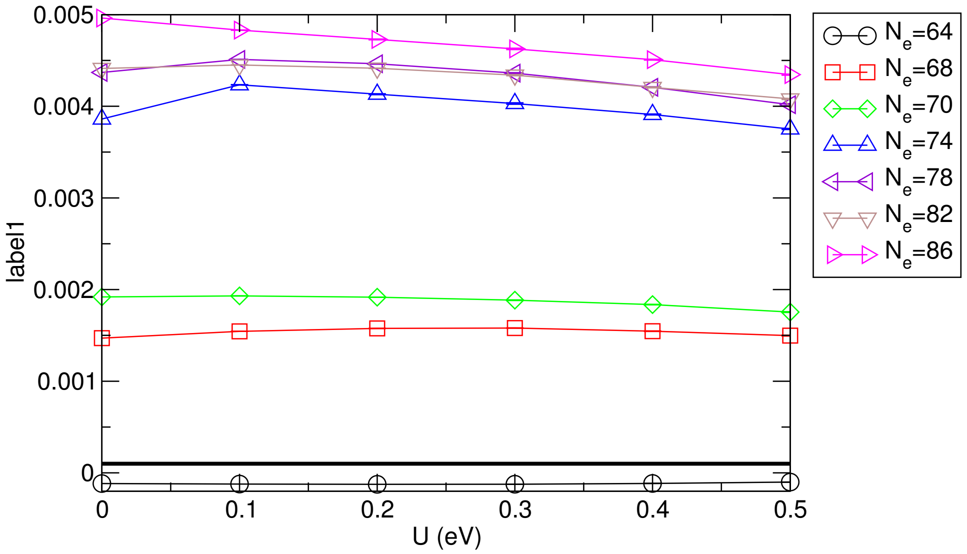


FIG. S32: CPMC average long-range pair-pair correlations for the 64 site lattice, X=CN, symmetry $d_4$. Absence of enhancement is seen for all $N_e$.

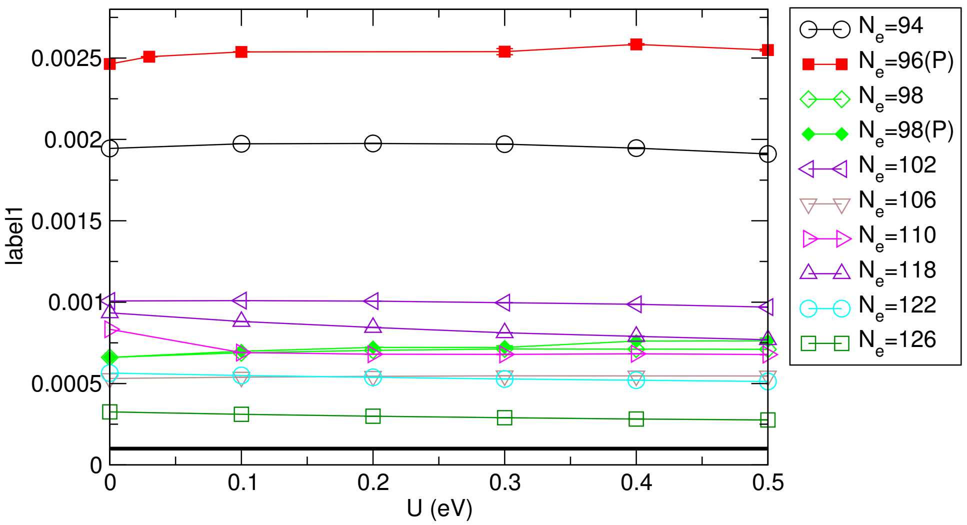


FIG. S33: CPMC average long-range pair-pair correlations for the 64 site lattice, X=CN, symmetry $d_4$. Absence of enhancement is seen for all $N_e$.
